# Supplementary material for: Data-efficient multi-fidelity training for high-fidelity machine learning interatomic potentials
Source: arXiv:2409.07947 ancillary file (2024-09-12)
Supplement: Supplementary file 1 [file Supplementary.pdf]

## Contents

- I. Test on model architecture
- II. MLIPs validation results for argyrodite  $\text{Li}_6\text{PS}_5\text{Cl}$
- III. Equilibrium mixing energy of  $\text{In}_x\text{Ga}_{1-x}\text{N}$
- IV. Benchmark results for ternary phase diagrams of SevenNet-MF-0
- V. Phonon band structures of SevenNet-MF-0
- VI. Data distribution of MP-r<sup>2</sup>SCAN database
- VII. Multi-fidelity MLIP for molecular systems with coupled cluster quality

References

## I. Test on model architecture

In machine learning, utilizing more parameters usually increases the model capability, resulting in better performance as long as using an abundant database. However, increasing fidelity-dependent parameters might hinder application of MLIPs since high-fidelity databases are scarce. For instance, those parameters might lead to overfitting rather than learning general information from learnable weights that are commonly used with a low-fidelity database, leading to worse generalizability of high-fidelity MLIPs. Therefore, we tested the generalizability of MLIPs by varying the model architecture. First, we train MLIPs using the multi-fidelity  $\text{In}_x\text{Ga}_{1-x}\text{N}$  database used in section 2.2. For high-fidelity databases, we utilize binary crystal configurations. First, we include only strained crystals in the high-fidelity database (named EOS-DB) and then include every binary configuration obtained from ab initio MD simulations (called C100). We train five models by varying the train and validation set split while training. Then, we compare energy, force and stress of the high-fidelity test set that contains MD trajectory of ternary alloys.

First, we tested by changing the atomic energy shifting and scaling scheme. Using different shift (scale) values on each database are labeled  $\text{DW}_{\text{shift}}$  ( $\text{DW}_{\text{scale}}$ ), which stands for database-wise shift (scale). We observe that a model not using  $\text{DW}_{\text{shift}}$  results in unacceptably high error in the training set, indicating the incapability of our multi-fidelity model without  $\text{DW}_{\text{shift}}$ . This can be interpreted by the different reference energy of each database, since this can be effectively solved by incorporating  $\text{DW}_{\text{shift}}$ . Therefore, we use  $\text{DW}_{\text{shift}}$  as default and analyze the effect of  $\text{DW}_{\text{scale}}$ . The generalizability of each model is illustrated in Supplementary Fig. 1. Results show using the same atomic energy scaling for both low- and high-fidelity databases gives robust accuracy toward out-of-distribution (OOD). This might be because utilizing  $\text{DW}_{\text{scale}}$  leads to using different energy units for each database, hindering the knowledge propagation from a low-fidelity database.

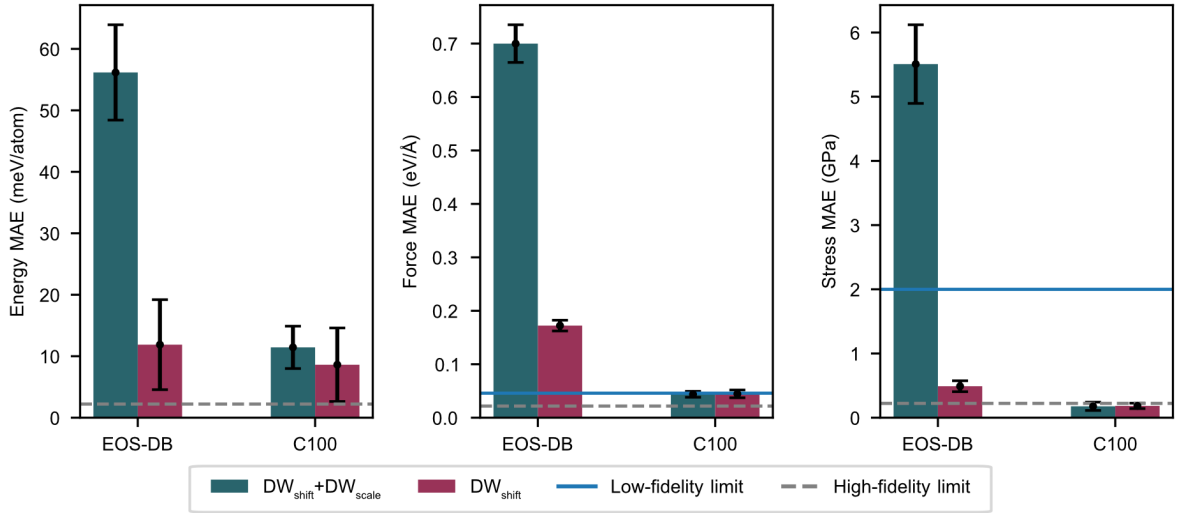

**Supplementary Fig. 1 | Bar plots showing energy, force and stress MAEs of MLIPs trained on the multi-fidelity database by varying atomic energy shifting and scaling schemes.** Each MLIP is trained using EOS-DB or C100 as a high-fidelity database. Blue line indicates the conventional error level of MLIP trained on single-fidelity database utilizing full low-fidelity data while gray dashed line shows the error limit of MLIP trained solely on full high-fidelity database. Error bars represent the standard deviation of MAEs for five MLIPs.

Next, we tested the model architecture related to modified linear layers. Modified linear layers that can be incorporated into original SevenNet are able to be classified as two categories: modified

element-dependent layer (MEL) and modified global layer (MGL). This criterion is based on the characteristics of each module, as MEL are related to the trainable parameters that are differently used for each element, while MGL are related to trainable parameters that are globally used, independent to the types of elements. MEL includes modified linear layers for an atom-type embedding block and MGL includes modified linear layers in interaction blocks and an output block. Results are represented in Supplementary Fig. 2. Figure shows only utilizing MGL gives the most robust results. In contrast, incorporating MEL gives worse generalizability, especially when using a small high-fidelity database. This might be interpreted as follows. Atom-type embedding vectors are an important feature of GNN MLIPs that encode the important chemical nature of each element. However, when using MEL, embedding vectors are different for each database, which might lead to inappropriate embedding vectors for a data-scarce high-fidelity database. This would hinder the high-fidelity MLIPs to learn appropriate chemical nature of each element, resulting in high error for unsampled In-Ga interaction in the test set. We use the best setting (only  $DW_{\text{shift}}$ ) for atomic energy shifting and scaling while testing MEL and MGL. We both use MEL and MGL when we initially testing  $DW_{\text{shift}}$  and  $DW_{\text{scale}}$ . Notably, MEL+MGL in Supplementary Fig. 2 are having the same model architecture with  $DW_{\text{shift}}$  in Supplementary Fig. 1.

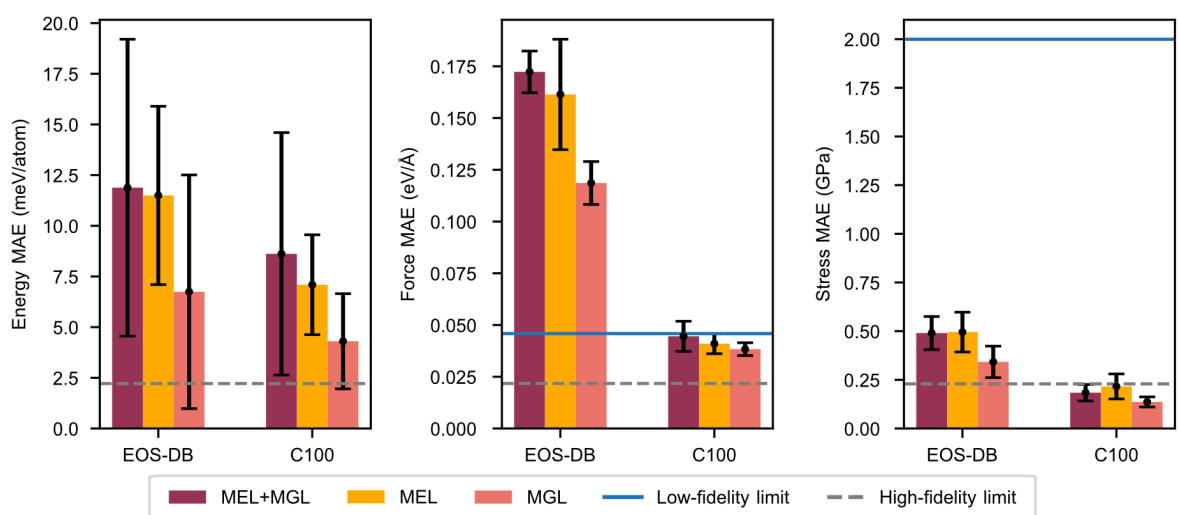

**Supplementary Fig. 2 | Bar plots showing energy, force and stress MAEs of MLIPs trained on the multi-fidelity database by changing the usage of modified linear layers in each module.** Each MLIP is trained using EOS-DB or C100 as a high-fidelity database. Blue line indicates the conventional error level of MLIP trained on single-fidelity database utilizing full low-fidelity data while gray dashed line shows the error limit of MLIP trained solely on full high-fidelity database. Error bars represent the standard deviation of MAEs for five MLIPs.

## II. MLIPs validation results for argyrodite $\text{Li}_6\text{PS}_5\text{Cl}$

The MLIP validation procedure used in ref. 1 includes the following process: 1) Lattice parameter and energy at equilibrium structure of  $\text{Li}_6\text{PS}_5\text{Cl}$  containing various disorder distributions, 2) MSD of lithium comparison between DFT and MLIP at  $\text{Li}_6\text{PS}_5\text{Cl}$  unit cell, and 3) checking energy error for MLIP-MD configurations with DFT single-point calculations. We follow this three steps validation procedure to MLIPs trained on  $\text{Li}_6\text{PS}_5\text{Cl}$  systems to validate the performance of our MLIPs.

First, we check the lattice parameter and energy of equilibrium  $\text{Li}_6\text{PS}_5\text{Cl}$  crystal structures. We utilize the unit cell structure to validate the MLIPs for argyrodite  $\text{Li}_6\text{PS}_5\text{Cl}$  with 0, 25, 50, 75 and 100% Cl@4c structure. For each structure, we construct 25 configurations that are having distinct disorder distributions. As demonstrated in Supplementary Fig. 3, it is evident that all MLIPs maintain high accuracy in calculating lattice parameters and total energy compared to DFT, regardless of disorder. Notably, lattice parameters calculated with PBE functional with 50% Cl@4c results in much higher value near 9.95 Å, exceeding the upper limit calculated with MLIPs. Supplementary Figure 3b reveals that the baseline MLIP underestimates the unit cell energy by approximately 5 meV/atom across all disorders. This systematic trend suggests that the discrepancy results from atomic-energy ad-hoc mapping. However, this does not necessarily imply that significant issues will arise during MD simulations.

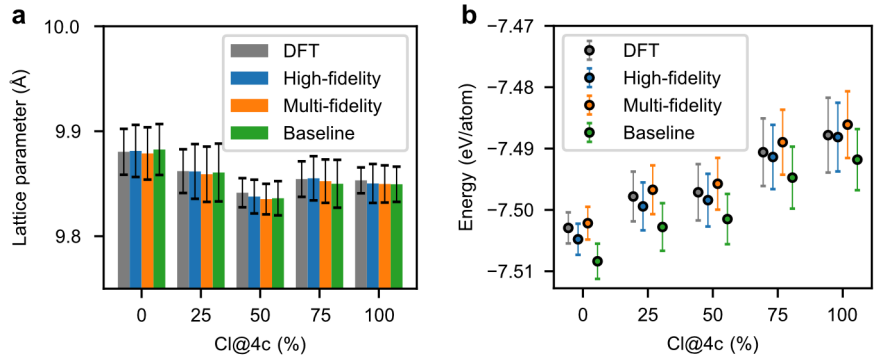

**Supplementary Fig. 3 | Comparison of ground-state properties of the unit cells of  $\text{Li}_6\text{PS}_5\text{Cl}$  calculated with DFT, reference high-fidelity MLIP, multi-fidelity MLIP and the baseline MLIP.** **a**, Lattice parameters and **b**, total energies obtained by 25 distinct cells per disorder ratio with DFT and each MLIP. Mean values are presented with standard deviations as error bars.

Next, we compare the MSD of Li-ions in the unit cell  $\text{Li}_6\text{PS}_5\text{Cl}$  between DFT and MLIPs. We utilize 0, 50 and 100% Cl@4c structure and conduct NVT simulation at 500 K for 100 ps. For MD employing MLIPs, we conduct 5 unit cell configurations with distinct disorder distributions. Supplementary Figure 4 shows that there is no significant difference in the MSD computed from ab initio MD simulations at 500 K for all MLIPs, included within the standard deviation.

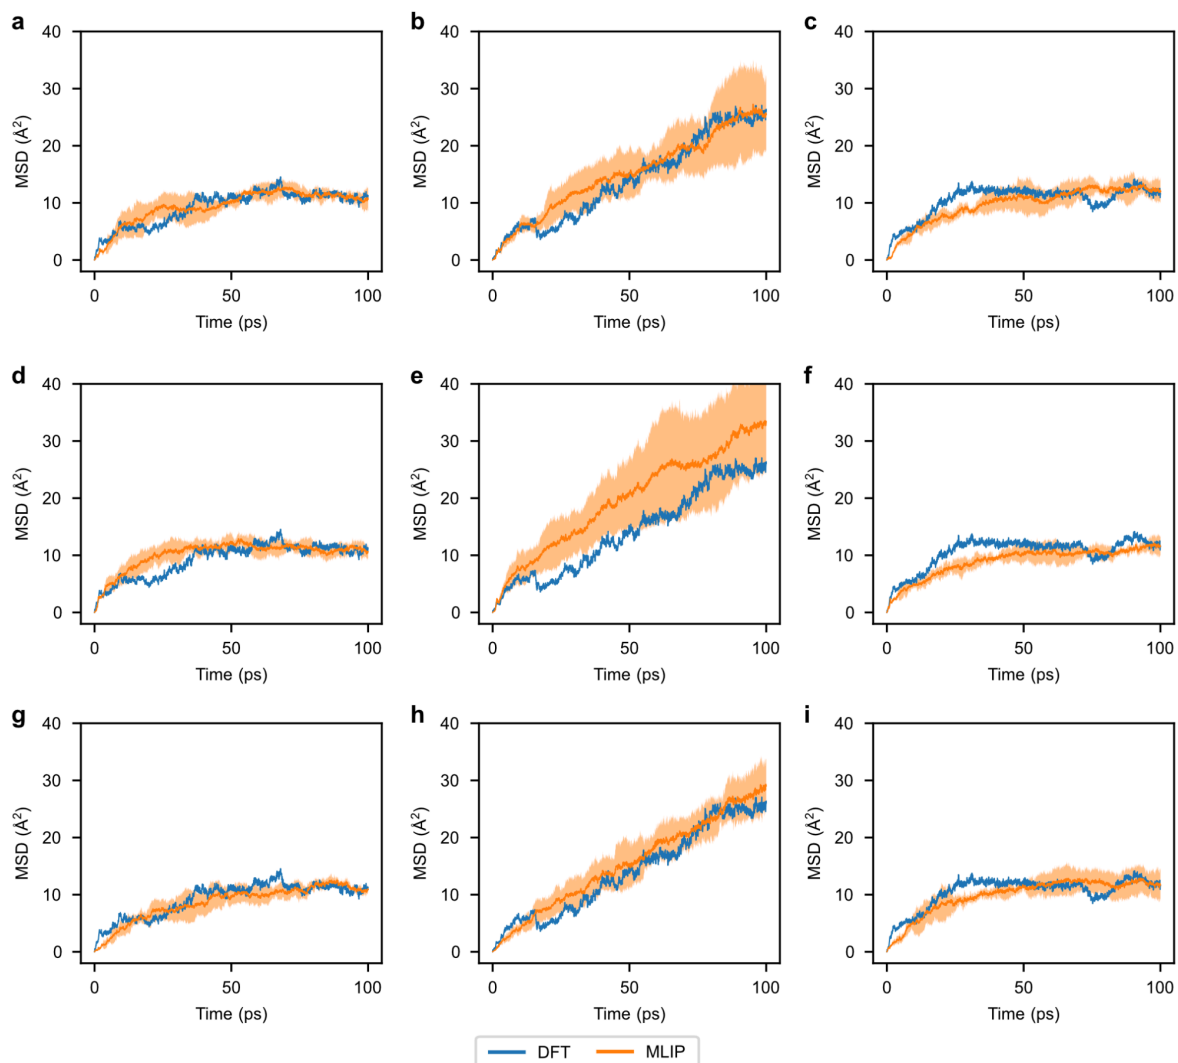

**Supplementary Fig. 4 | MSD plots of DFT and MLIP at 500 K MD simulations in the unit cells of  $\text{Li}_6\text{PS}_5\text{Cl}$ .** From the first column to the last one, they represent 0, 50 and 100% Cl@4c unit cells, respectively. **a–c**, MSD plots calculated using reference high-fidelity MLIP, **d–f**, MSD plots calculated using multi-fidelity MLIP, and **g–h**, MSD plots calculated using the baseline MLIP compared with DFT MD. Shaded regions for MLIPs show standard deviation depending on disorder distribution.

Finally, we validate MLIPs by comparing energy using DFT single-point calculations for MLIP-MD trajectories. We conduct 2 ns NVT simulations using each MLIP at 300, 600 and 700 K. Results in 300 K indicate high prediction accuracy, as observed in Supplementary Fig. 5a–c. Conversely, Supplementary Fig. 5f demonstrates significant energy discrepancies in the baseline MLIP results when performing MD simulations at 600 K. This discrepancy arises due to the emergence of unphysical short Li-Li bonds during the MLIP-MD simulations. In contrast, such phenomena are not observed when conducting MD simulations with the reference high-fidelity MLIP and multi-fidelity MLIP. This trend consistently appears even at 700 K MLIP-MD, as shown in Supplementary Figures 5g–i. This indicates that, unlike the high- and multi-fidelity MLIP, the baseline MLIP has limitations for conducting MD simulations at temperatures above 600 K.

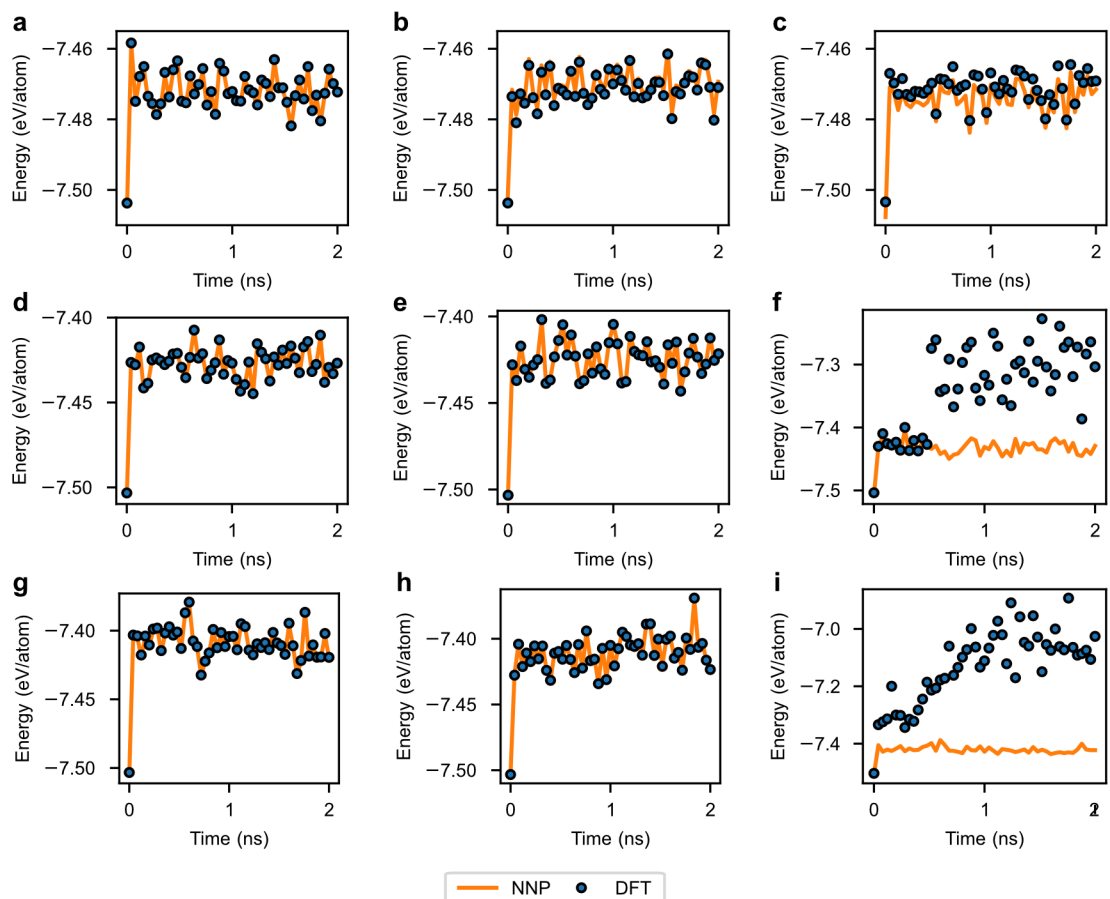

**Supplementary Fig. 5 | Energy plots of MLIP-MD simulation and DFT single-point calculation with SCAN functional in 50% Cl@4c unit cell.** From the first column to the last one, they represent the results of reference high-fidelity MLIP, multi-fidelity MLIP, and the baseline MLIP, respectively. **a–c**, Energies of 300 K MLIP-MD trajectory. **d–f**, Energies of 600 K MLIP-MD trajectory. **g–i**, Energies of 700 K MLIP-MD trajectory.

### III. Equilibrium mixing energy of $\text{In}_x\text{Ga}_{1-x}\text{N}$

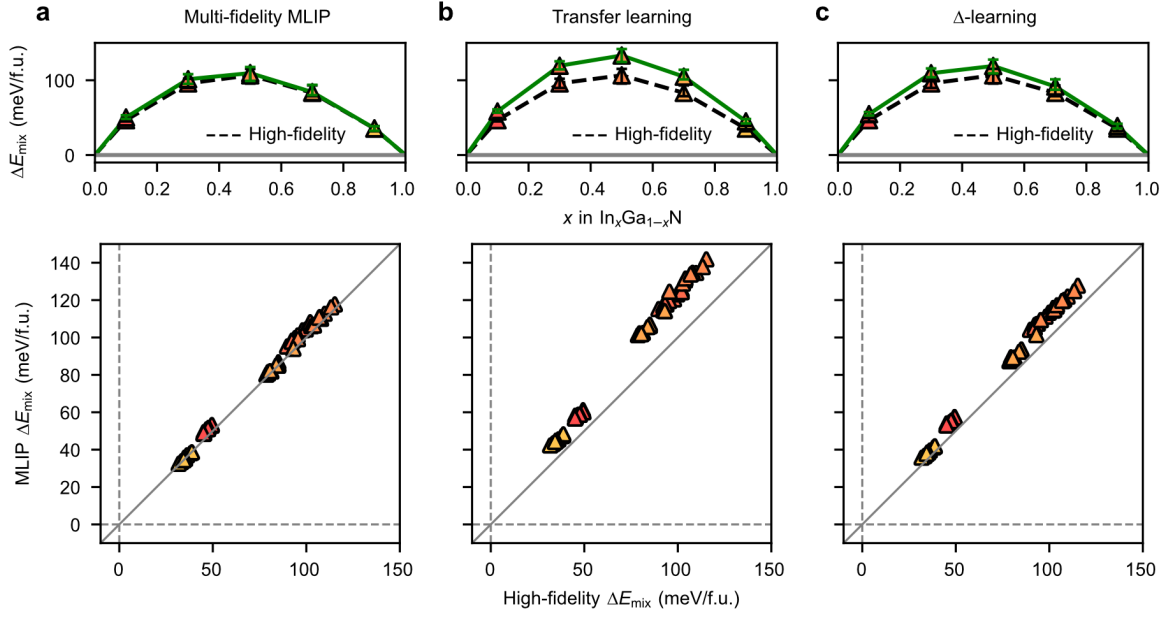

**Supplementary Fig. 6 | Mixing energies of fully relaxed alloys calculated with each MLIP training method.** **a**, (Top) Average mixing energies and their range (error bars) for 10 random alloys and (Bottom) parity plot showing correlation to reference high-fidelity MLIP with MLIP trained with multi-fidelity approach. **b**, Similar results obtained by transfer learning and **c**,  $\Delta$ -learning.

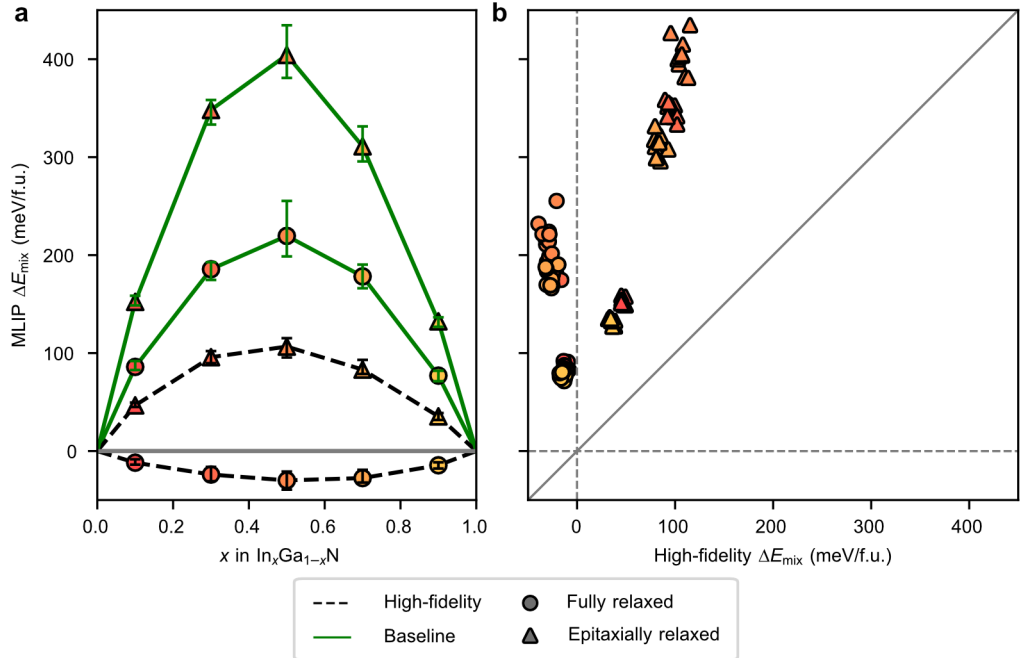

**Supplementary Fig. 7 | Equilibrium mixing energy of baseline MLIP compared with reference high-fidelity MLIP.** **a**, Average mixing energies along compositions while error bars show the range of mixing energies. **b**, Parity plot showing mixing energy of individual alloys.

#### IV. Benchmark results for ternary phase diagrams of SevenNet-MF-0

We further evaluate SevenNet-MF-0 on ternary systems involving oxides, nitrides, and fluorides, which are particularly valuable for constructing phase diagrams using the  $r^2$ SCAN functional without requiring empirical energy corrections as in PBE (+U)<sup>2</sup>. We focus on systems where the stable binary and ternary compositions differ significantly between  $r^2$ SCAN and PBE (+U), using phase data from the Materials Project<sup>3</sup>. Some phases missing in the  $r^2$ SCAN calculations are excluded from the  $r^2$ SCAN phase diagram. The results are shown in Supplementary Fig. 8 and 9. SevenNet-MF-0 demonstrates good alignment with the  $r^2$ SCAN phase diagrams, accurately predicting stable and unstable compounds, though with a few notable discrepancies. These differences could stem from the lower resolution of SevenNet-MF-0 or missing competing phases in the  $r^2$ SCAN phase diagram. For example, in the Li-Zr-O system,  $Zr_4O$  is above the hull by 8 meV/atom in SevenNet-MF-0, while  $r^2$ SCAN predicts it to be stable. In the Ce-Se-N system, SevenNet-MF-0 predicts  $Ce_{10}Se_{19}$  as a stable phase, rather than  $CeSe_2$ , which is missing in the  $r^2$ SCAN phase diagram.

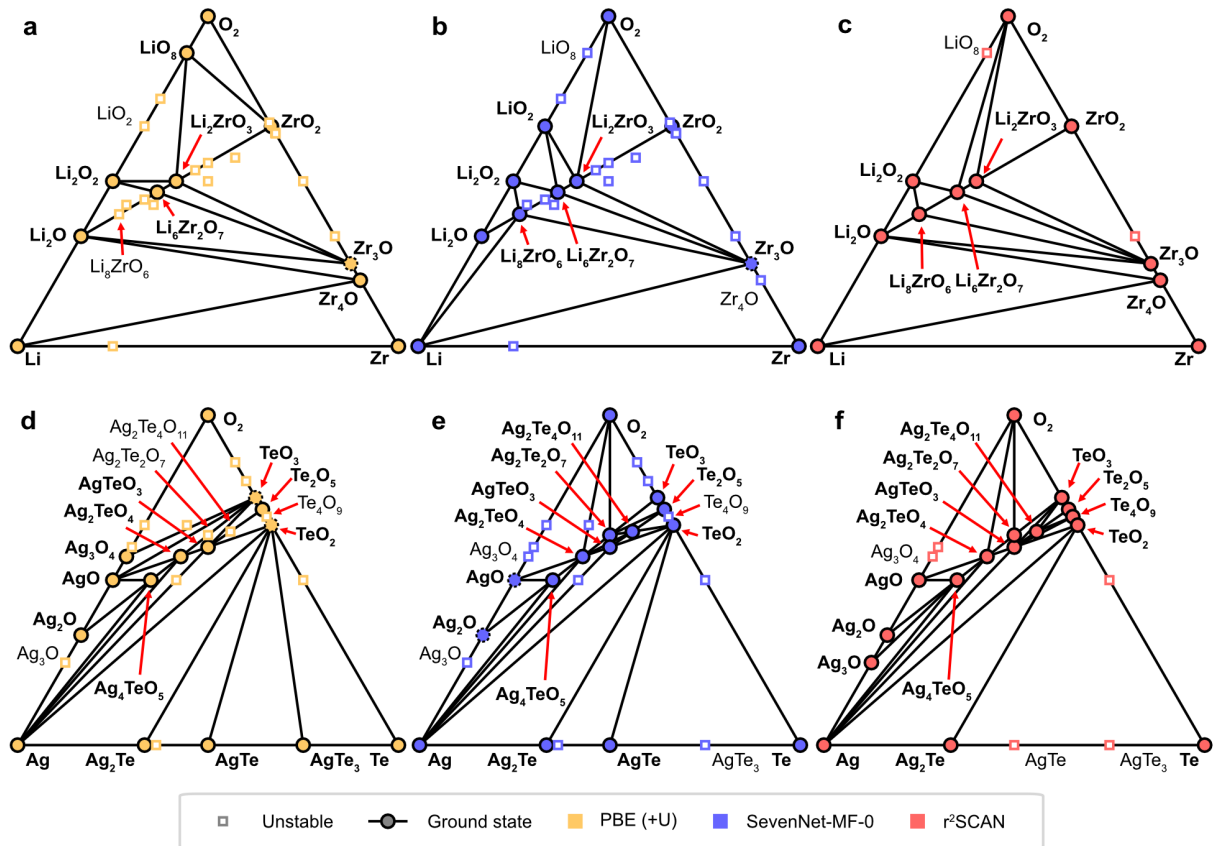

**Supplementary Fig. 8 | Phase diagrams for benchmark oxide (Li-Zr-O and Ag-Te-O) systems.** From the first column to the last one, they represent the phase diagrams constructed using PBE (+U), SevenNet-MF-0 and  $r^2$ SCAN, respectively. **a–c**, Phase diagrams of Li-Zr-O system, **d–f**, phase diagrams of Ag-Te-O system. Dashed circles in **a** ( $Zr_3O$ ) and **d** ( $TeO_3$ ,  $TeO_2$ ) represent the PBE (+U) ground state compounds that show discrepancies with  $r^2$ SCAN. Similarly, dashed circles in **b** ( $Zr_3O$ ) and **e** ( $AgO$ ,  $Ag_2O$ ) show the cases for SevenNet-MF-0.

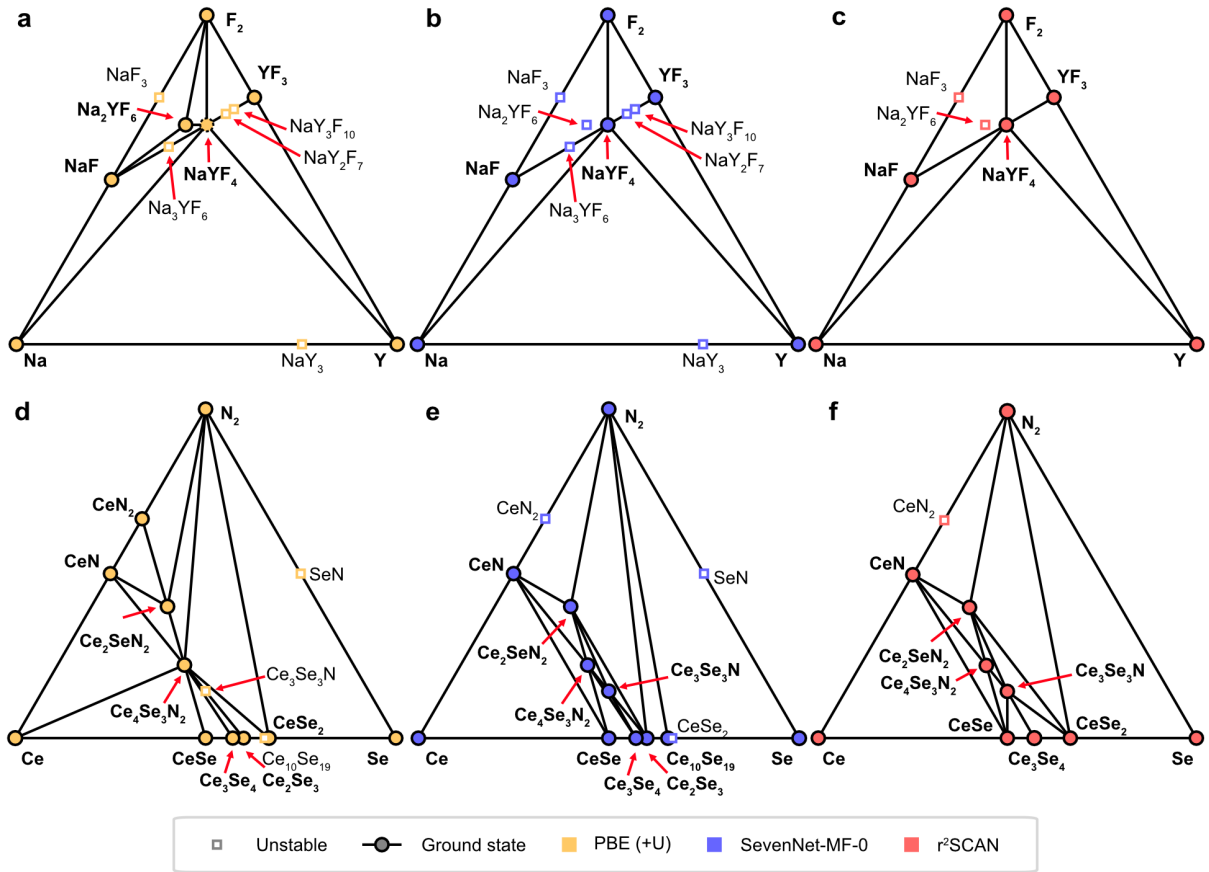

**Supplementary Fig. 9 | Phase diagrams for benchmark fluoride (Na-Y-F) and nitride (Ce-Se-N) systems.** From the first column to the last one, they represent the phase diagrams constructed using PBE (+U), SevenNet-MF-0 and r<sup>2</sup>SCAN, respectively. **a–c**, Phase diagrams of Na-Y-F system, **d–f**, phase diagrams of Ce-Se-N system. Dashed circle in **a** (Na<sub>2</sub>YF<sub>6</sub>) represents the case where PBE (+U) predicts different crystal structure as a ground state with r<sup>2</sup>SCAN.

## V. Phonon band structures of SevenNet-MF-0

Phonon band structures calculated with SevenNet-MF-0, SevenNet-0 and  $r^2$ SCAN functional are represented in Supplementary Fig. 10, where  $r^2$ SCAN phonon band structures are obtained from refs. 4,5. We observe that both SevenNet-0 and SevenNet-MF-0 can qualitatively reproduce phonon band structures but underestimate the phonon frequencies, especially for optical phonons. We also found SevenNet-MF-0 predicts softer phonon structures than SevenNet-0, regardless of whether the material actually exhibits softer phonon in PBE (Si, GaAs, NiO, MgO, and CaO) or  $r^2$ SCAN (Fe).

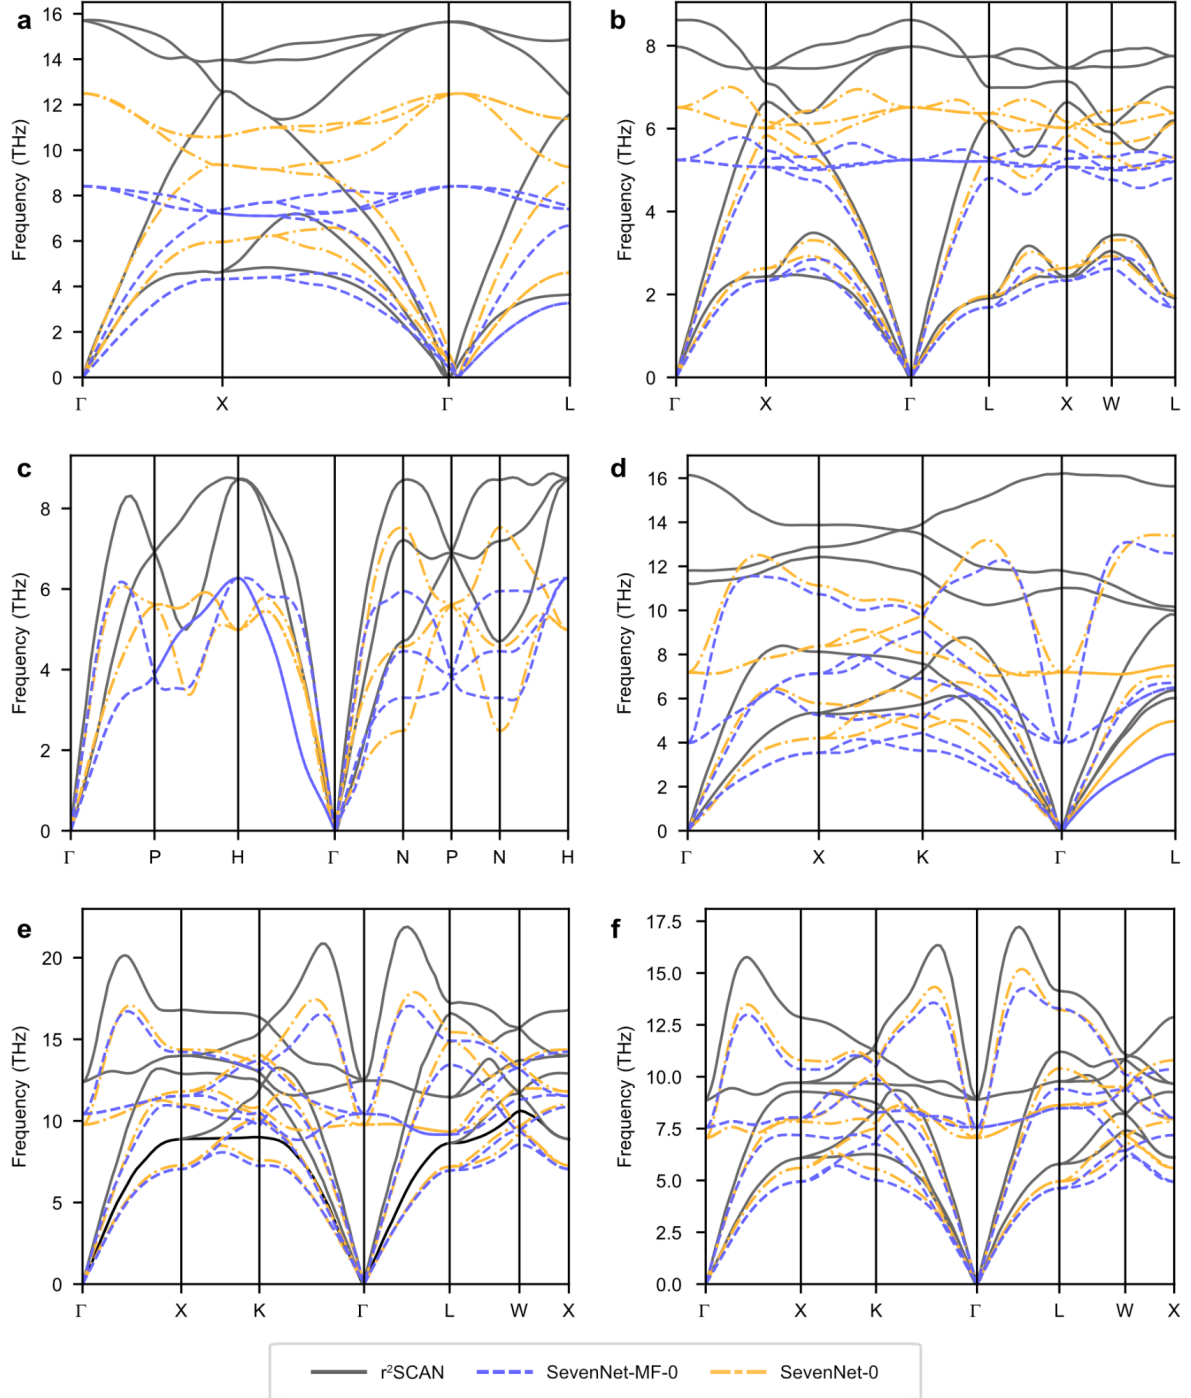

**Supplementary Fig. 10 | Phonon band structures for benchmark unary and binary materials.** Phonon structures for **a**, Si, **b**, GaAs, **c**, Fe, **d**, NiO, **e**, MgO, and **f**, CaO.

## VI. Data distribution of MP-r<sup>2</sup>SCAN database

Here, we demonstrate the data distribution of MP-r<sup>2</sup>SCAN database, mainly compared with MPF.2021.2.8 database<sup>3,6</sup>. We first compare the chemical characteristics of each database. The number of elements used in MPF.2021.2.8 and MP-r<sup>2</sup>SCAN are compared in Supplementary Fig. 11a. The portion of each element in each database is showing similar trends such as oxygen has the highest occupation, noble gas and radioactive elements (e.g. Tc, Pm and Ac) are occupying very low portions. Notably, Yb is not included in the MP-r<sup>2</sup>SCAN database, resulting in 89 elements in the MPF.2021.2.8 database and 88 elements in the MP-r<sup>2</sup>SCAN database. We further analyze the crystals by categorizing based on the number of composing elements. As illustrated in Supplementary Fig. 11b, MP-r<sup>2</sup>SCAN database contains up to ternary composition. On the other hand, MPF.2021.2.8 database includes a broader chemical environment by encompassing crystals up to octonary systems (e.g. NaAl<sub>6</sub>Fe<sub>3</sub>Si<sub>6</sub>B<sub>3</sub>H<sub>3</sub>O<sub>30</sub>F, mp-863003).

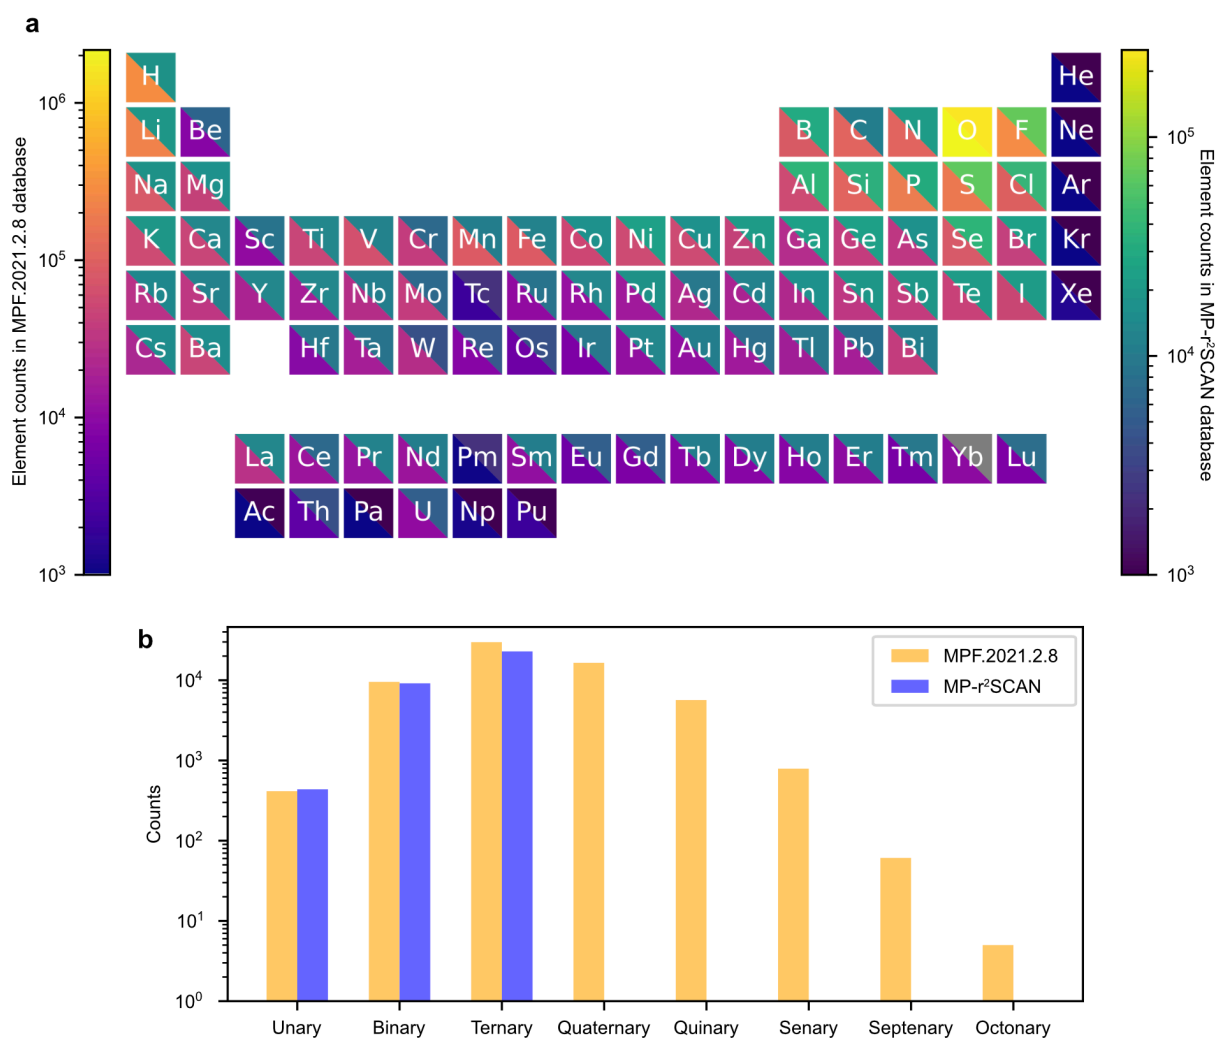

**Supplementary Fig. 11 | Chemical distribution of databases provided in the Materials Project. a,** Periodic table representing the element distribution of MPF.2021.2.8 and MP-r<sup>2</sup>SCAN database. Distribution in MPF.2021.2.8 is located as the lower left part of each element while MP-r<sup>2</sup>SCAN database is located as upper-left triangles. Elements missing in the database are colored in gray (Yb in MP-r<sup>2</sup>SCAN). **b,** Compounds distribution by the number of elements in each crystal structure.

Next, we compare the energy, force and stress distribution of each database. Direct comparison of total energy provided in each database is meaningless, since the energy reference of each database varies. Therefore, we compare formation energy and energy above the hull (in PBE (+U) scheme) provided by the Materials Project. Supplementary Figure 12a,b shows statistical distribution of formation energy and energy above the hull near zero. It shows that the portion of stable compounds in the MP-r<sup>2</sup>SCAN database are higher than the MPF.2021.2.8 database, resulting in significant undersampling of high-energy polymorphs. This is because the Materials Project mainly applies r<sup>2</sup>SCAN calculation to the crystals with high stability, as stated in ref. 2. Next, we compare the force and stress distribution of each database. To represent the scale of force and stress, we calculate the norm of force and von Mises stress for each configuration. Supplementary Figure 12c,d illustrates that the MP-r<sup>2</sup>SCAN database contains significantly smaller force and stress compared to the MPF.2021.2.8 database. This is because relaxation trajectories in high-fidelity databases are started from DFT equilibrium obtained from low-fidelity calculations<sup>7</sup>, resulting in narrowly ranged force and stress near zero.

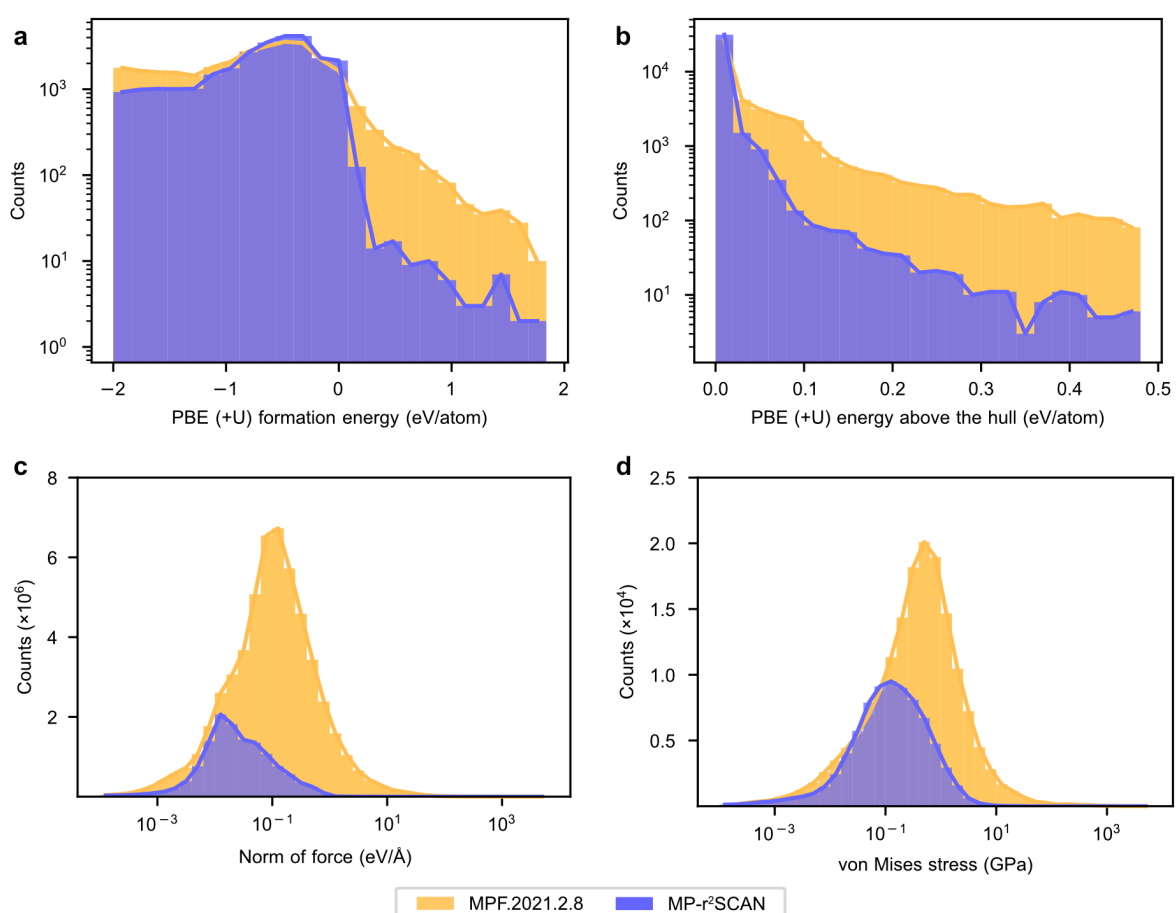

**Supplementary Fig. 12 | Histograms representing energy, force and stress distribution of databases provided in the Materials Project.** Distribution of **a**, formation energy, **b**, energy above the hull, **c**, norm of force and **d**, von Mises stress for each fidelity database. Formation energy and energy above the hull values are retrieved from the Materials Project based on material identification numbers of each distinct compound in the databases. Few materials that do not provide formation energy and energy above the hull data are excluded. Norm of force and von Mises stress are calculated for every atom and structure provided by each database.

## VII. Multi-fidelity MLIP for molecular systems with coupled cluster quality

First, we assess the performance of MLIPs trained on ethanol datasets by comparing the errors in predicted energy and forces to the reference CCSD(T) energy and forces on a test set of 500 ethanol configurations, which were excluded from the training data. We train SevenNet on 1,000 configurations from the DFT dataset, and as a baseline, we also train a model on 100 randomly chosen configurations from the CCSD(T) dataset. Finally, we develop a multi-fidelity model by training SevenNet on both the 1,000 DFT and 100 CCSD(T) configurations. Since DFT energy consistently shifts relative to CCSD(T) energy, we compare relative energies, defined as the total energy minus the energy of the most stable configuration, rather than comparing absolute values. The parity plots of relative energy and force are provided in Supplementary Fig. 13. Our findings show that MLIP trained on DFT energy and forces underperforms due to the lower fidelity of the training set, while the baseline model lacks accuracy because of insufficient data. In contrast, the multi-fidelity model accurately predicts CCSD(T) energy and forces by leveraging information from both low- and high-fidelity datasets.

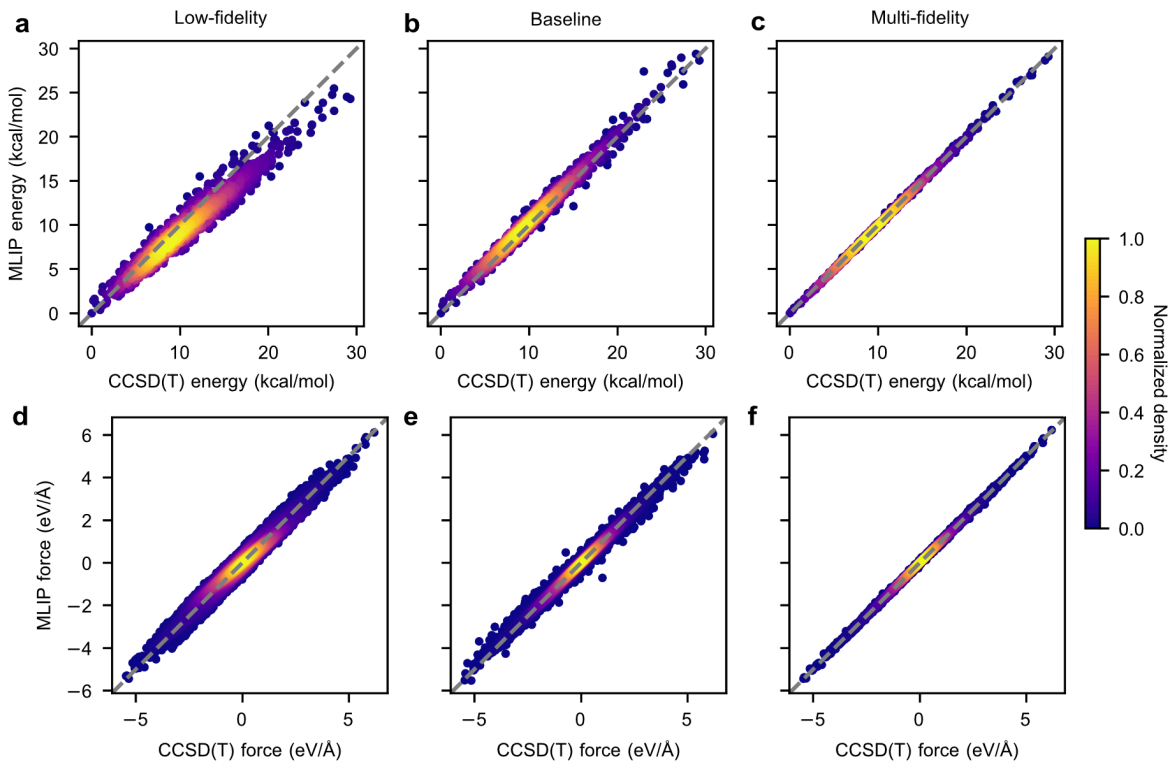

**Supplementary Fig. 13 | Parity plots showing energy and force correlations between CCSD(T) calculation and MLIPs on ethanol test set.** From the first column to the last one, they represent the results of low-fidelity MLIP, baseline MLIP and multi-fidelity MLIP. **a–c**, Parity plots for relative energy and **d–f**, parity plots for force.

Second, we compare the potential energy surfaces (PES) of ethanol by rotating the hydroxyl group. Using each MLIP, we fully relax the ethanol molecule, constraining only the dihedral angle of the hydroxyl group. PES of each MLIP are illustrated in Supplementary Fig. 14. The multi-fidelity MLIP closely tracks the CCSD(T) PES, accurately predicting the ground state conformer. The MLIP trained

on DFT data follows the DFT PES and incorrectly identifies the gauche conformation as the ground state. Meanwhile, the baseline MLIP predicts the trans conformation as the ground state but shows poor agreement with the CCSD(T) PES. The PES for CCSD(T) and DFT are sourced from ref. 8.

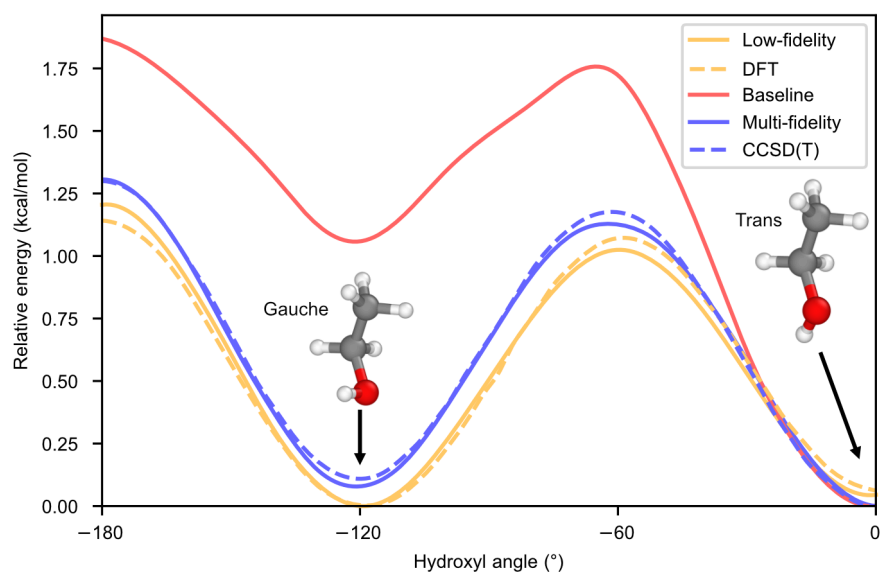

**Supplementary Fig. 14 | Potential energy surfaces of ethanol molecule, measured with various methods.** Solid lines represent PESs calculated with MLIPs while dashed lines indicate PESs calculated with ab initio methods. Local minimum near  $-120^\circ$  and  $0^\circ$  corresponds to gauche and trans conformer, respectively.

We perform similar experiments on the aspirin molecule and observe results consistent with those for ethanol in terms of energy and force predictions, as shown in Supplementary Fig. 15. As with the PES scanning of ethanol, we also generate a 2D PES for aspirin by rotating the dihedral angles of the ester and carboxylic acid groups. The results of 2D PES are represented in Supplementary Fig. 16a–d. The MLIP trained on DFT data shows a shallower rotational barrier compared to the high-fidelity MLIP trained on 1,000 CCSD aspirin configurations. This aligns with the findings in ref. 8, which used sGDML as the MLIP model. The multi-fidelity model closely matches the high-fidelity PES while using only one-tenth of the CCSD data. In contrast, the baseline MLIP results in unphysical PES, demonstrating that the success of the multi-fidelity model is due to knowledge transferred from the DFT database. Additionally, we conduct 500 ps NVT MD simulations at 300 K using each MLIP. The joint dihedral angle distribution of ester and carboxylic acid groups while MD simulations are illustrated in Supplementary Fig. 16e–i. The MD trajectory shows that the low-fidelity MLIP (trained on DFT data) results in more frequent functional group rotations due to the shallower rotational barrier, while the multi-fidelity MLIP accurately reproduces the dihedral angle distribution of the high-fidelity MLIP by correctly predicting the barrier.

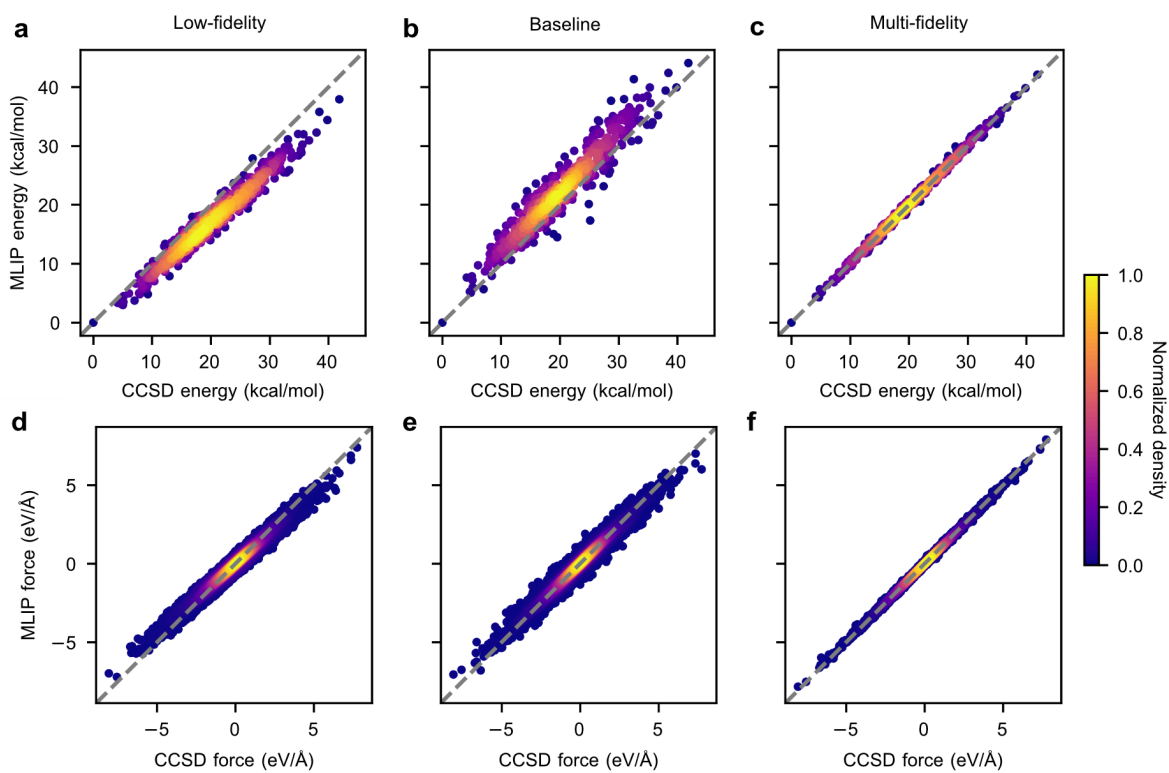

**Supplementary Fig. 15 | Parity plots showing energy and force correlations between CCSD calculation and MLIPs on aspirin test set.** From the first column to the last one, they represent the results of low-fidelity MLIP, baseline MLIP and multi-fidelity MLIP. **a–c**, Parity plots for relative energy and **d–f**, for force.

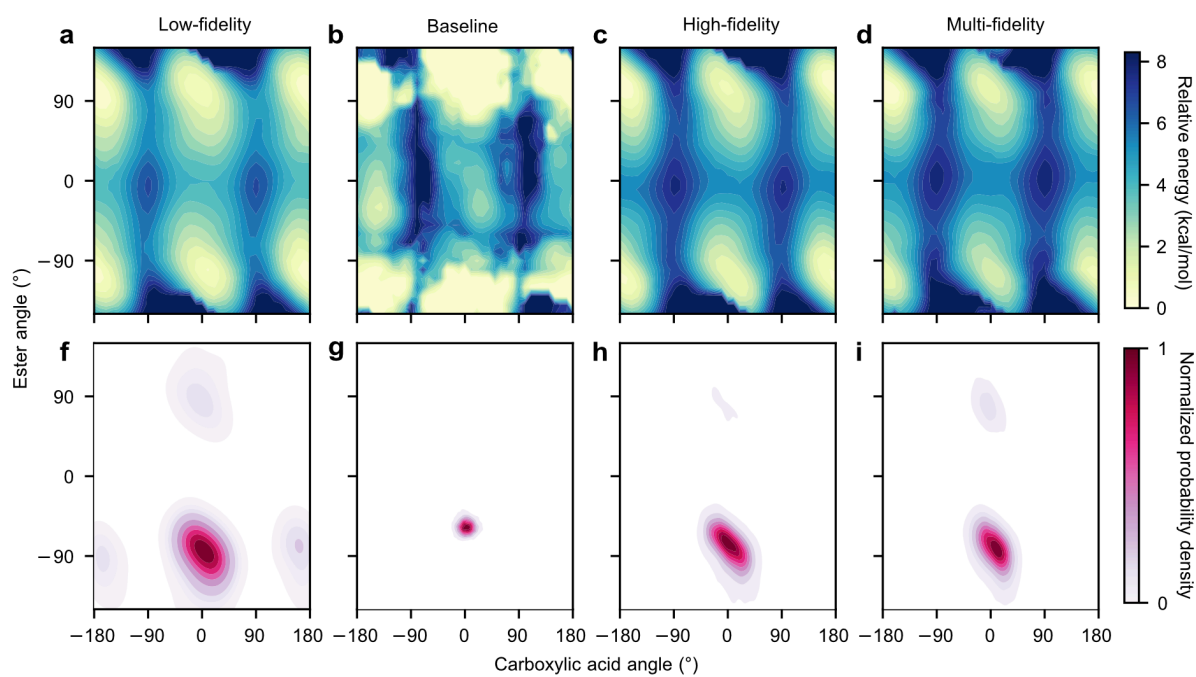

**Supplementary Fig. 16 | Potential energy surfaces and dihedral angle distributions of aspirin molecule measured by various MLIPs.** From the first column to the last one, they represent the results of low-fidelity MLIP, baseline MLIP, high-fidelity MLIP and multi-fidelity MLIP. **a–c**, PES scanned by rotating ester and carboxylic acid groups. **d–f**, Probability density of joint angle distribution.

## References

1. Lee, J. *et al.* Disorder-dependent Li diffusion in  $\text{Li}_6\text{PS}_5\text{Cl}$  investigated by machine-learning potential. *ACS Appl. Mater. Interfaces* **16**, 46442–46453 (2024).
2. Kingsbury, R. S. *et al.* A flexible and scalable scheme for mixing computed formation energies from different levels of theory. *npj Comput. Mater.* **8**, 1–11 (2022).
3. Jain, A. *et al.* Commentary: The Materials Project: A materials genome approach to accelerating materials innovation. *APL Mater.* **1**, 011002 (2013).
4. Ning, J., Furness, J. W. & Sun, J. Reliable lattice dynamics from an efficient density functional approximation. *Chem. Mater.* (2022).
5. Lee, K., Park, Y. & Han, S. *Ab initio* construction of full phase diagram of MgO-CaO eutectic system using neural network interatomic potentials. *Phys. Rev. Mater.* **6**, 113802 (2022).
6. Chen, C. & Ong, S. P. A universal graph deep learning interatomic potential for the periodic table. *Nat. Comput. Sci.* **2**, 718–728 (2022).
7. Kingsbury, R. *et al.* Performance comparison of  $r^2\text{SCAN}$  and SCAN metaGGA density functionals for solid materials via an automated, high-throughput computational workflow. *Phys. Rev. Mater.* **6**, (2022).
8. Chmiela, S., Sauceda, H. E., Müller, K.-R. & Tkatchenko, A. Towards exact molecular dynamics simulations with machine-learned force fields. *Nat. Commun.* **9**, 1–10 (2018).
